# Supplementary material for: Sealed-bid Auctions on Blockchain with Timed Commitment Outsourcing
Source: arXiv:2410.10607 source file (2026-10-19)
Supplement: Supplementary file 1 [file Appendix.tex]

\section*{Appendix}

\section{Proof of Lemma~\ref{lemma:group}}
\label{proof:lemma-group}

\section{Correctness and Security Analysis of Aggregable Timed Commitment} \label{appendix:ATLP}

\section{Proof of Theorem~\ref{thm:bne}}
\label{proof:thm-bne}

\section{Proof of Theorem~\ref{thm:sym}}
\label{proof:thm-sym}

\section{Proof for Theorem~\ref{thm:hbw}}

\section{Proof of Theorem~\ref{thm:two-side-DSIC}}
\label{proof:thm-two-side-DSIC}

% \textbf{Remark. }In other cases where the value distribution $F$ is limited to the distribution set with zero support at values smaller than $\underline{V}$, the expected revenue of a two-side DSIC mechanism cannot reach a positive fraction of the revenue of our mechanism. That is, our the ratio of its revenue and the revenue of our mechanism can approach to infinity. For example, let $g(x)=x$ and the value distribution is $U[\underline{V},\overline {V}]$. Then for any two-side DSIC mechanism, the computing cost shouldn't exceed $\underline{V}$. 

% Consider the distribution $U[\frac{\underline{V}} k,\frac{\overline {V}} k]$. It's easy to observe that the ratio is not sensitive to the positive scaling $k$. Let $\overline V=k$ grows to infinity, our revenue is approximately the one running on distribution $U[0,1]$, which is strictly positive. while the above discussion shows the revenue(certainly smaller than welfare) of this two-sides DSIC mechanism approach to zero.

% The ratio will be no larger than 
% \begin{align}
% &(\text{Denote $\max_i{v_i}$ as $v_{max}$})\\
% &\quad\frac
% {E_{\vec {v},\vec l}[v_{max}*(\underline{v}*\max_jl_j)]}{rev}
% \\&= \frac{E_{\vec {v},\vec l}[v_{max}^2]}
% {E_{\vec {v},\vec l}[v_{max}*\underline{v}]}
% \\&\ge \frac{E_{\vec {v},\vec l}[v_{max}]}
% {\underline{v}}
% \ge \frac{\underline{v}+\overline{v}}{2\underline{v}}
% \end{align}
